# Supplementary material for: Lipizzaner: A System That Scales Robust Generative Adversarial Network Training
Source: arXiv:1811.12843 source file (2018-11-30)
Supplement: Supplementary file 1 [file appendix.tex]

\appendix
\section{\horse Algorithm}
\label{sec:horse-algorithm}

The \horse behavior on one gradient-based GAN trainer is described in
detail in Program~\ref{alg:lippizaner}.

\begin{algorithm*}
  \small
  \caption{\texttt{Lipizzaner}: 
    {\small
    Evolve distributed populations of
    generators $\mathcal{G}$ and discriminators $\mathcal{D}$, the
    hyperparameters and mixture weights, $\omega$.\newline    
    \textbf{Input:}\newline 	
    \protect\begin{tabular}{ll}  
    ~$T$~: Number of iterations &~$E$~: Grid cells \\
    ~$k$~: Neighborhood size & ~$\theta_{COEV}$~: Parameters for \texttt{stepGANCoev}
    \protect\end{tabular}
    }
  }
  \label{alg:lippizaner}
  \begin{algorithmic}[1]
    
    \ParFor{$c \in E$} \Comment{Asynchronous parallel execution of all cells in grid}
    \State $t \gets 0$
    \State $n, \omega \gets$ initializeNeighborhoodAndMixtureWeights($c, k$) \Comment{Uniform initialization of settings}
    \For{$t \leq T$} \Comment{Iterations}
    \State $n, \omega \gets$ \texttt{stepGANCoev}($n, \omega, \theta_{COEV}$) \Comment{ Coevolve GAN using Alg. \ref{alg:gan-coev}}
    \State $n, \omega \gets$ calculateGANMixtureMeasure($n, \omega$) \Comment{Calculate Inception score for mixture}
    \State $t \gets t + 1$
    \EndFor
    \EndParFor
    \State \Return $(n, \omega)^*$ \Comment{ Cell with best generator mixture } 
  \end{algorithmic}
\end{algorithm*}

\begin{algorithm*}
  \small
  \caption{\texttt{stepGANCoev}:
    { \small
    Evolve distributed populations of
    generators $\mathcal{G}$ and discriminators $\mathcal{D}$ and the
    hyperparameters $\alpha, \omega$.\newline
    \textbf{Input:}\newline
    \protect\begin{tabular}{llll}   
    ~$n$~: Cell neighborhood & ~$\omega$~: Neighbor weight &~$\gamma$~: Replacement size  & ~$X$~: Input dataset \\
    ~$\beta, \mu$~: Mutation probabilities & ~$\tau$~: Tournament size & ~$\alpha$~: Learning rate
    \protect\end{tabular}
    }
  }\label{alg:gan-coev}
  \begin{algorithmic}[1]
    \State $n' \gets$ select($n, \tau$) \Comment{ Select based on fitness ($\mathcal{L}$) }
    \State $\mathbf{B} \gets $ getMiniBatches($X$) \Comment{ Load minibatchs }
    \For{$B \in \mathbf{B}$} \Comment{Loop over batches}
    \State $\alpha \gets$ mutateLearningRate($\alpha, \beta$) \Comment{ Update with with gaussian mutation }
    \State \Comment{Generator}
    \For{$G \in n_G'$} \Comment{Update generators}
    \State $D \gets$ getRandomOpponent($n_D', \omega_D$) \Comment{ Get weighted uniform random discriminator}
    \State $\nabla_{G} \gets$ computeGradient($G, D, \alpha_G$) \Comment{ Compute gradient for neighborhood center }
    \State $G \gets$ updateNN($G, \nabla_G, B$) \Comment{ Update with gradient }
    \EndFor
    \State \Comment{Discriminator}
    \For{$D \in n_D'$} \Comment{Update discriminator}
    \State $G \gets$ getRandomOpponent($n_G', \omega_G$) \Comment{ Get weighted uniform random generator}
    \State $\nabla_{D} \gets$ computeGradient($D, G, \alpha_D$) \Comment{ Compute gradient for neighborhood center }
    \State $D \gets$ updateNN($D, \nabla_D, B$) \Comment{ Update with gradient }
    \EndFor
    \EndFor
    
    \State $\omega_D' \gets $ mutate$(\omega_D, \mu)$ \Comment{Gaussian mutation of discriminator mixture weights }
    \State $\omega_G' \gets $ mutate$(\omega_G, \mu)$ \Comment{Gaussian mutation of generator mixture weights }

    \For{$G, D \in n_G' \times n_D'$} \Comment{Evalute GANs}
    \State $\mathcal{L}_{D,G} \gets$ evaluate($D, G, B$) \Comment{ Evaluate GAN on batch}
    \EndFor

    \State $n_D \gets \max(n_D', n_D)$ \Comment{ Replace if new discriminator fitness is better}
    \State $n_G \gets \max(n_G', n_G)$ \Comment{ Replace if new generator fitness is better}
    \State \Return $n, \omega$
  \end{algorithmic}
\end{algorithm*}

\section{Experimental settings}

\begin{table}
  \centering
  \caption{Setup for experiments conducted with the coevolutionary,
    gradient-based \horse algorithm.}
  \label{tbl:exp-lpz}
  \begin{tabular}{|l|l|}
    \hline
    \multicolumn{2}{|l|}{\textbf{Coevolutionary settings}} \\ \hline
    Generations & 30 (1600 batches each) \\ \hline
    Population size per cell & 1 \\ \hline
    Tournament size & 2 \\ \hline
    Grid size & 1x1, 2x2 \\ \hline
    Mixture size & 0.01 (learning rate) \\ \hline
    \multicolumn{2}{|l|}{\textbf{Hyperparameter mutation}} \\ \hline
    Optimizer & Adam \\ \hline
    Initial learning rate & 0.002 \\ \hline
    Mutation rate & 0.0001 \\ \hline
    Mutation probability & 0.5 \\ \hline
    \multicolumn{2}{|l|}{\textbf{Network topology}} \\ \hline
    Network type  & DCGAN \\ \hline
    Input neurons & 100 \\ \hline
    Number of hidden layers & 4 (convolutional) \\ \hline
    Neurons per hidden layer & 16,384 $-$ 131,072 \\ \hline
    Output neurons  & 64x64x3 (RGB pixels) \\ \hline
    Activation function & $tanh$ \\ \hline
    & \textbf{CelebA} \\ \hline
  \end{tabular}
\end{table}
